# Supplementary material for: Efficient Progressive Image Compression with Variance-aware Masking
Source: arXiv:2411.10185 source file (2025-01-10)
Supplement: Supplementary file 1 [file additional.tex]

\section{Additional results }
\vspace{-0.5cm}
Fig. \ref{fig:mssim} compares our method with other progressive models regarding \emph{Multiscale  structural similarity index measure} (MS-SSIM) \cite{ssim} on Kodak. While slightly outperformed by Jeon overall, we maintain complexity improvements noted in the main manuscript.
Part of the future work will be to focus on perceptual metrics.
Fig. \ref{fig:mask_analysis} shows the distribution of the bpps against the quality of the reconstruction in terms of the mean squared error (MSE) when varying $q$.
As is evident, at lower bitrates, the length of the bitstream increases exponentially with the chosen percentile values $q$ used to generate progressive masks.
This trend is logical because initially we include points with higher standard deviations, which contain more information but require more bits for storage.
In contrast, as $q$ increases and approaches the maximum value (100), only points with a lower standard deviation are omitted, which however have minimal impact on the final bitstream.
Figures \ref{com_cpu} (a,b) show GFLOPs and the time to decode using a CPU on Kodak.

\begin{figure}[!h]
%\begin{minipage}[b]{1.0\linewidth} 
  \centering
 \includegraphics[width=0.65\columnwidth]{images/5_additional/results_mssm.pdf}
 % \vspace{0.1cm}
  \caption{bbp vs. MS-SSIM curve against existing progressive sotas models on Kodak: Proposed, Jeon, Lee, and JPEG2000. }
  \label{fig:mssim}
%\end{minipage}
\end{figure}

\begin{figure}[h!]
%\begin{minipage}[b]{1.0\linewidth} 
  \centering
 \includegraphics[width=0.60\columnwidth]{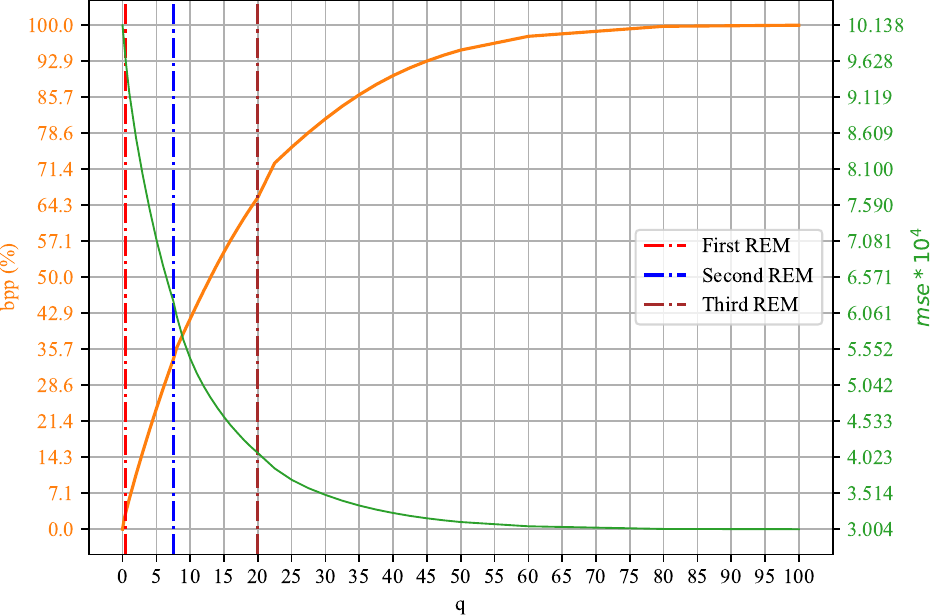}
 % \vspace{0.1cm}
  \caption{Distribution of the bpps (orange) and MSE (green) when varying $q$ on Kodak.}
  \label{fig:mask_analysis}
%\end{minipage}
\end{figure}

\begin{figure}[t]
    \centering
    \begin{minipage}[b]{0.30\textwidth}
        \centering
        \includegraphics[width=0.80\textwidth]{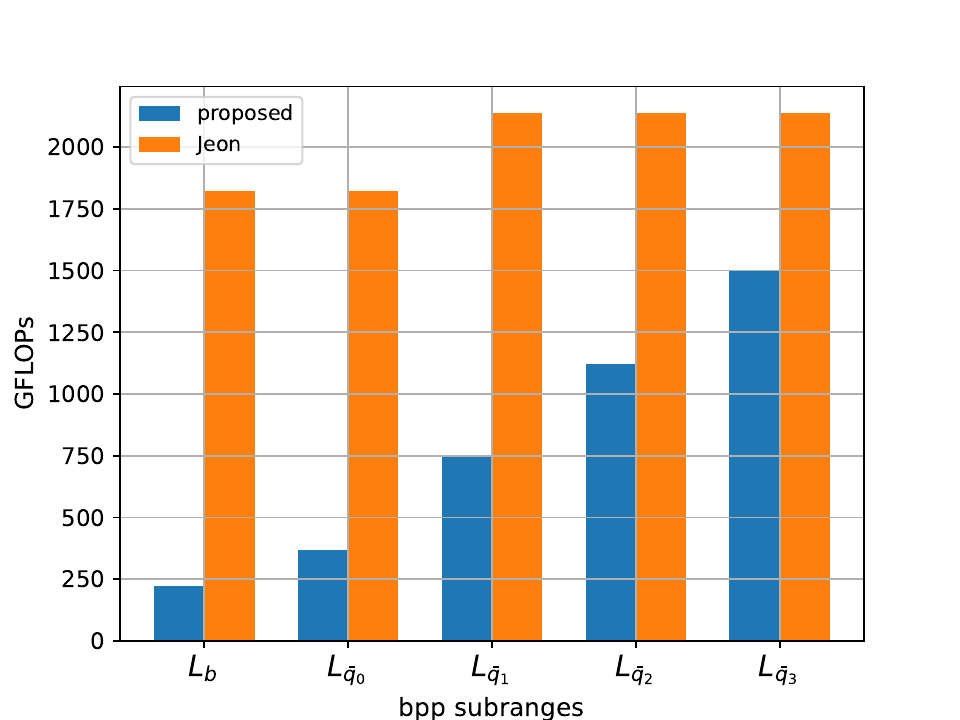}
        \subcaption{ }
        \label{fig:com1}
    \end{minipage}
    \vspace{-0.25cm}
    \begin{minipage}[b]{0.30\textwidth}
        \centering
        \includegraphics[width=0.80\textwidth]{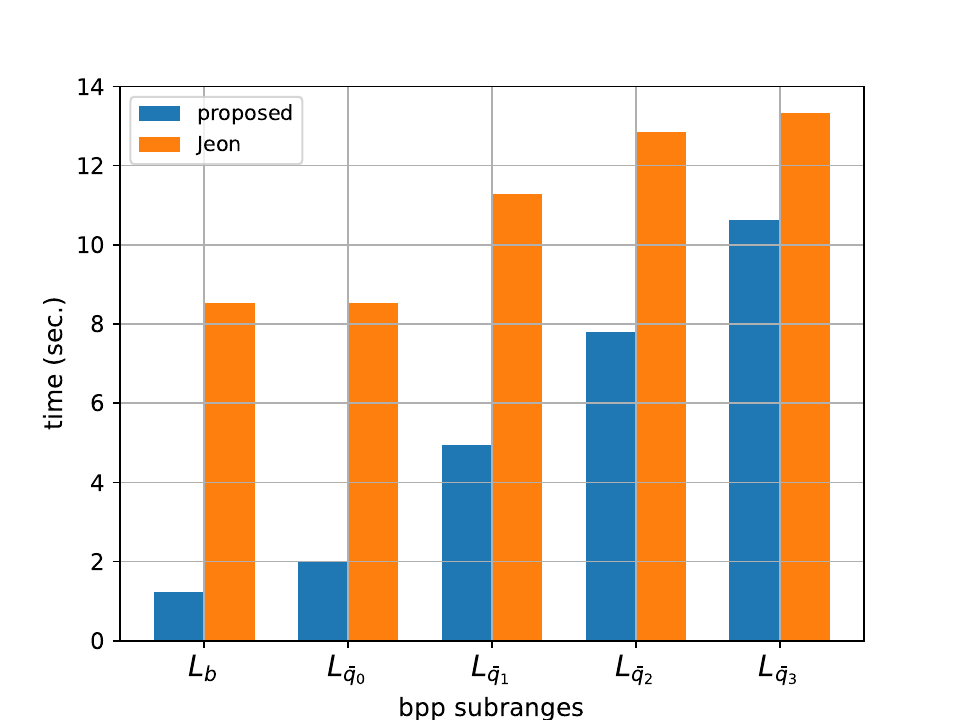}
        \subcaption{}
        \label{fig:com2}
    \end{minipage}
    \caption{GFLOPs and decoding time complexity on CPU (a,b)  vs.\ Jeon~\emph{et~al.}, considering different subranges on Kodak.}
    \label{com_cpu}
\end{figure}

\begin{figure*}[!b]
    \centering
    \begin{minipage}{0.8\textwidth}
        \centering
        % Riga 1
        \begin{minipage}{0.3\textwidth}
            \centering
            \includegraphics[width=\linewidth]{images/5_additional/kodim07/original.pdf}
            \subcaption{Input: bpp/PSNR/ \% of bpp}
        \end{minipage}\hfill
        \begin{minipage}{0.3\textwidth}
            \centering
            \includegraphics[width=\linewidth]{images/5_additional/kodim07/base.pdf}
            \subcaption{\emph{base}: 0.16/32.93/37}
        \end{minipage}\hfill
        \begin{minipage}{0.3\textwidth}
            \centering
            \includegraphics[width=\linewidth]{images/5_additional/kodim07/05.pdf}
            \subcaption{$q$=0.5:0.17/32.25/39.5}
        \end{minipage}
        
        \vspace{0.5cm} % Spazio tra le righe
        
        % Riga 2
        \begin{minipage}{0.3\textwidth}
            \centering
            \includegraphics[width=\linewidth]{images/5_additional/kodim07/kod_10.pdf}
            \subcaption{$q$=10:0.32/35.62/74}
        \end{minipage}\hfill
        \begin{minipage}{0.3\textwidth}
            \centering
            \includegraphics[width=\linewidth]{images/5_additional/kodim07/kod_25.pdf}
            \subcaption{$q$=25: 0.38/36.84/88 }
        \end{minipage}\hfill
        \begin{minipage}{0.3\textwidth}
            \centering
            \includegraphics[width=\linewidth]{images/5_additional/kodim07/kod_100.pdf}
            \subcaption{$q$=10: 0.43/37.48/100}
        \end{minipage}
    \end{minipage}
    \caption{Reconstruction of Kodim07 from kodak dataset using proposed method.}
    \label{fig:kodim07}
\end{figure*}

Figures \ref{fig:kodim07},\ref{fig:kodim23} are  image reconstruction from Kodak.
Figures \ref{fig:main},\ref{fig:main2} are from CLIC validation dataset, with some latent representations across various qualities.

\begin{figure*}[]
    \centering
    \begin{minipage}{0.8\textwidth}
        \centering
        % Riga 1
        \begin{minipage}{0.3\textwidth}
            \centering
            \includegraphics[width=\linewidth]{images/5_additional/kodim23/or.pdf}
            \subcaption{Input: bpp/PSNR/ \% of bpp}
        \end{minipage}\hfill
        \begin{minipage}{0.3\textwidth}
            \centering
            \includegraphics[width=\linewidth]{images/5_additional/kodim23/base.pdf}
            \subcaption{\emph{base}: 0.096/33.33/34}
        \end{minipage}\hfill
        \begin{minipage}{0.3\textwidth}
            \centering
            \includegraphics[width=\linewidth]{images/5_additional/kodim23/kod_05.pdf}
            \subcaption{$q$=0.5:0.109/33.79/41.9}
        \end{minipage}
        
        \vspace{0.5cm} % Spazio tra le righe
        
        % Riga 2
        \begin{minipage}{0.3\textwidth}
            \centering
            \includegraphics[width=\linewidth]{images/5_additional/kodim23/kod_10.pdf}
            \subcaption{$q$=10:0.22/37.40/84.6}
        \end{minipage}\hfill
        \begin{minipage}{0.3\textwidth}
            \centering
            \includegraphics[width=\linewidth]{images/5_additional/kodim23/kod25.pdf}
            \subcaption{$q$=25: 0.24/37.89/92.3 }
        \end{minipage}\hfill
        \begin{minipage}{0.3\textwidth}
            \centering
            \includegraphics[width=\linewidth]{images/5_additional/kodim23/kod_100.pdf}
            \subcaption{$q$=10: 0.26/37.96/100}
        \end{minipage}
    \end{minipage}
    \caption{Reconstruction of Kodim23 from kodak dataset using proposed method.}
    \label{fig:kodim23}
\end{figure*}

\begin{figure*}[!h]
    \centering
    \begin{minipage}[t]{0.7\textwidth}
        \centering
        % Big image
        \includegraphics[width=1\textwidth]{images/5_additional/schika/or/input.pdf}
        \subcaption{Input image}
        \vfill
        \begin{minipage}[t]{0.3\textwidth}
            \centering
            \includegraphics[width=\textwidth]{images/5_additional/schika/base/std_base_258.png}
            \subcaption{Base std}
        \end{minipage}
        \hfill
        \begin{minipage}[t]{0.3\textwidth}
            \centering
            \includegraphics[width=\textwidth]{images/5_additional/schika/base/ch_base_258.png}
            \subcaption{Base channel}
        \end{minipage}
        \hfill
        \begin{minipage}[t]{0.3\textwidth}
            \centering
            \includegraphics[width=\textwidth]{images/5_additional/schika/base/crop_0.08_34.21.png}
            \subcaption{Rec. (0.08,34.14)}
        \end{minipage}

    \end{minipage}
    \vfill
    \begin{minipage}[t]{0.7\textwidth}
        \centering
        \begin{minipage}[t]{0.24\textwidth}
            \centering
            \includegraphics[width=\textwidth]{images/5_additional/schika/0.5/mask_0.05_258.png}
            \subcaption{mask at $q$=0.5}
        \end{minipage}
        \hfill
        \begin{minipage}[t]{0.24\textwidth}
            \centering
            \includegraphics[width=\textwidth]{images/5_additional/schika/0.5/std_0.05_258.png}
            \subcaption{std at $q$=0.5}
        \end{minipage}
        \hfill
        \begin{minipage}[t]{0.24\textwidth}
            \centering
            \includegraphics[width=\textwidth]{images/5_additional/schika/0.5/ch_0.05_258.png}
            \subcaption{channel at $q$=0.5}
        \end{minipage}
        \hfill 
        \begin{minipage}[t]{0.24\textwidth}
            \centering
            \includegraphics[width=\textwidth]{images/5_additional/schika/0.5/crop_0.09_34.54.png}
            \subcaption{Rec (0.09,34.54)}
        \end{minipage}
        \hfill

        \begin{minipage}[t]{0.24\textwidth}
            \centering
            \includegraphics[width=\textwidth]{images/5_additional/schika/7.5/mask_0.5_258.png}
            \subcaption{mask at $q$=7.5}
        \end{minipage}
        \hfill
        \begin{minipage}[t]{0.24\textwidth}
            \centering
            \includegraphics[width=\textwidth]{images/5_additional/schika/7.5/std_0.5_258.png}
            \subcaption{std at $q$=7.5}
        \end{minipage}
        \hfill
        \begin{minipage}[t]{0.24\textwidth}
            \centering
            \includegraphics[width=\textwidth]{images/5_additional/schika/7.5/ch_0.5_258.png}
            \subcaption{channel at $q$=7.5}
        \end{minipage}
        \begin{minipage}[t]{0.24\textwidth}
            \centering
            \includegraphics[width=\textwidth]{images/5_additional/schika/7.5/crop_0.18_37.15.png}
            \subcaption{Rec. (0.18,37.15)}
        \end{minipage}

        \vfill
        \begin{minipage}[t]{0.24\textwidth}
            \centering
            \includegraphics[width=\textwidth]{images/5_additional/schika/20/l_20_258.png}
            \subcaption{Mask at $q$=20}
        \end{minipage}
        \hfill
        \begin{minipage}[t]{0.24\textwidth}
            \centering
            \includegraphics[width=\textwidth]{images/5_additional/schika/20/std_20_258.png}
            \subcaption{std at $q$=20}
        \end{minipage}
        \hfill
        \begin{minipage}[t]{0.24\textwidth}
            \centering
            \includegraphics[width=\textwidth]{images/5_additional/schika/20/ch_20_258.png}
            \subcaption{channel at $q$=20}
        \end{minipage}
        \begin{minipage}[t]{0.24\textwidth}
            \centering
            \includegraphics[width=\textwidth]{images/5_additional/schika/20/crop_0.21_38.04.png}
            \subcaption{Rec. (0.21,38.04)}
        \end{minipage}
        \vfill

        \begin{minipage}[t]{0.3\textwidth}
            \centering
            \includegraphics[width=\textwidth]{images/5_additional/schika/100/ch_10_258.png}
            \subcaption{Std at $q$=100 (top).}
        \end{minipage}
        \hfill
        \begin{minipage}[t]{0.3\textwidth}
            \centering
            \includegraphics[width=\textwidth]{images/5_additional/schika/100/tl_10_258.png}
            \subcaption{channel at $q$=100 (top)}
        \end{minipage}
        \hfill
        \begin{minipage}[t]{0.3\textwidth}
            \centering
            \includegraphics[width=\textwidth]{images/5_additional/schika/100/crop_0.23_38.30.png}
            \subcaption{Rec. (0.23,38.3)}
        \end{minipage}
    \end{minipage}
    \caption{Final reconstruction with latent representations for different qualities, which varies through the raws.}\label{fig:main}
\end{figure*}

%%%%%%%%%%%%%%%%%%%%%%% LATENTS 2 %%%%%%%%%%%%%%%%%%%%%%%%%%%%
\begin{figure*}[!h]
    \centering
    \begin{minipage}[t]{0.7\textwidth}
        \centering
        % Big image
        \includegraphics[width=1\textwidth]{images/5_additional/roberto/or/input_rob.pdf}
        \subcaption{Input image}
        \vfill
        \begin{minipage}[t]{0.3\textwidth}
            \centering
            \includegraphics[width=\textwidth]{images/5_additional/roberto/or/std_base_258.png}
            \subcaption{Base std}
        \end{minipage}
        \hfill
        \begin{minipage}[t]{0.3\textwidth}
            \centering
            \includegraphics[width=\textwidth]{images/5_additional/roberto/or/ch_base_258.png}
            \subcaption{Base channel}
        \end{minipage}
        \hfill
        \begin{minipage}[t]{0.3\textwidth}
            \centering
            \includegraphics[width=\textwidth]{images/5_additional/roberto/base/crop_0.05_35.45.png}
            \subcaption{Rec. (0.05,35.45)}
        \end{minipage}

    \end{minipage}
    \vfill
    \begin{minipage}[t]{0.7\textwidth}
        \centering
        \begin{minipage}[t]{0.24\textwidth}
            \centering
            \includegraphics[width=\textwidth]{images/5_additional/roberto/0.5/m_0.05_258.png}
            \subcaption{mask at $q$=0.5}
        \end{minipage}
        \hfill
        \begin{minipage}[t]{0.24\textwidth}
            \centering
            \includegraphics[width=\textwidth]{images/5_additional/roberto/0.5/ch_0.05_258.png}
            \subcaption{std at $q$=0.5}
        \end{minipage}
        \hfill
        \begin{minipage}[t]{0.24\textwidth}
            \centering
            \includegraphics[width=\textwidth]{images/5_additional/roberto/0.5/tl_0.05_258.png}
            \subcaption{channel at $q$=0.5}
        \end{minipage}
        \hfill 
        \begin{minipage}[t]{0.24\textwidth}
            \centering
            \includegraphics[width=\textwidth]{images/5_additional/roberto/0.5/crop_0.06_35.92.png}
            \subcaption{Rec (0.06,35.92)}
        \end{minipage}
        \hfill

        \begin{minipage}[t]{0.24\textwidth}
            \centering
            \includegraphics[width=\textwidth]{images/5_additional/roberto/10/mask_1_258.png}
            \subcaption{mask at $q$=10}
        \end{minipage}
        \hfill
        \begin{minipage}[t]{0.24\textwidth}
            \centering
            \includegraphics[width=\textwidth]{images/5_additional/roberto/10/ch_1_258.png}
            \subcaption{std at $q$=10}
        \end{minipage}
        \hfill
        \begin{minipage}[t]{0.24\textwidth}
            \centering
            \includegraphics[width=\textwidth]{images/5_additional/roberto/10/ch_1_258.png}
            \subcaption{channel at $q$=10}
        \end{minipage}
        \begin{minipage}[t]{0.24\textwidth}
            \centering
            \includegraphics[width=\textwidth]{images/5_additional/roberto/10/crop_0.13_38.81.png}
            \subcaption{Rec. (0.13,38.81)}
        \end{minipage}

        \vfill
        \begin{minipage}[t]{0.24\textwidth}
            \centering
            \includegraphics[width=\textwidth]{images/5_additional/roberto/15/l_1.5_258.png}
            \subcaption{Mask at $q$=15}
        \end{minipage}
        \hfill
        \begin{minipage}[t]{0.24\textwidth}
            \centering
            \includegraphics[width=\textwidth]{images/5_additional/roberto/15/std_1.5_258.png}
            \subcaption{std at $q$=15}
        \end{minipage}
        \hfill
        \begin{minipage}[t]{0.24\textwidth}
            \centering
            \includegraphics[width=\textwidth]{images/5_additional/roberto/15/ch_1.5_258.png}
            \subcaption{channel at $q$=15}
        \end{minipage}
        \begin{minipage}[t]{0.24\textwidth}
            \centering
            \includegraphics[width=\textwidth]{images/5_additional/roberto/15/crop_0.14_38.86.png}
            \subcaption{Rec. (0.14,38.86)}
        \end{minipage}
        \vfill

        \begin{minipage}[t]{0.3\textwidth}
            \centering
            \includegraphics[width=\textwidth]{images/5_additional/roberto/100/std_10_258.png}
            \subcaption{Std at $q$=100 (top).}
        \end{minipage}
        \hfill
        \begin{minipage}[t]{0.3\textwidth}
            \centering
            \includegraphics[width=\textwidth]{images/5_additional/roberto/100/ch_10_258.png}
            \subcaption{channel at $q$=100 (top)}
        \end{minipage}
        \hfill
        \begin{minipage}[t]{0.3\textwidth}
            \centering
            \includegraphics[width=\textwidth]{images/5_additional/roberto/100/crop_0.142_38.886.png}
            \subcaption{Rec. (0.142,38.88)}
        \end{minipage}
    \end{minipage}
    \caption{Final reconstruction with latent representations for different qualities, which varies through the raws.}\label{fig:main2}
\end{figure*}
